# Supplementary material for: Predicting generalization performance with correctness discriminators
Source: arXiv:2311.09422 source file (2025-05-21)
Supplement: Supplementary file 1 [file llama_parser_sem.tex]

\begin{table*}[tb!]\centering
\footnotesize
\begin{tabularx}{\linewidth}{XXXXXXXXXXX}
\toprule
& \multicolumn{8}{c}{OOD} & \multicolumn{2}{c}{ID} \\
\cmidrule(lr){2-9}
\cmidrule(lr){10-11}
&\multicolumn{2}{c}{MCD1} &\multicolumn{2}{c}{MCD2} &\multicolumn{2}{c}{COGS} &\multicolumn{2}{c}{TOP} &\multicolumn{2}{c}{AMR 2.0} \\\cmidrule{2-11}
&Acc &AE $\downarrow$ &Acc &AE $\downarrow$&Acc &AE $\downarrow$&Acc &AE $\downarrow$ &Acc &AE $\downarrow$\\\midrule
{\textit{Ours(T5)}} \\\midrule
Single &52.2 &3.9 &31.6 &6.2 &86.6 &1.5 &70.6 &6.1 &7.1 &5.0 \\
Upper. & \textcolor{mdgreen}{59.9} &- & \textcolor{mdgreen}{41.2} &- & \textcolor{mdgreen}{87.9} &- & \textcolor{mdgreen}{78.0} &- & \textcolor{mdgreen}{13.6}&- \\
Lower. & \textcolor{mdgreen}{46.2} &- & \textcolor{mdgreen}{21.9} &- & \textcolor{mdgreen}{84.8} &- & \textcolor{mdgreen}{61.7} &- & \textcolor{mdgreen}{3.3} &- \\
Mean &53.0 &3.1 &31.6 &6.2 &86.3 &1.3 &69.8 &5.3 &8.4 &3.9 \\\midrule
{\textit{Ours(Vicuna)}} \\\midrule
Single &58.1 &0.3 &41.3 &15.9 &86.0 &0.9 &74.3 &9.8 &14.3 &5.8 \\
Upper. &\textcolor{mdgreen}{66.1} &- &\textcolor{red}{48.3} &- &\textcolor{mdgreen}{87.0} &- &\textcolor{mdgreen}{90.1} &- &\textcolor{mdgreen}{36.8} &- \\
Lower. &\textcolor{mdgreen}{49.6} &- &\textcolor{red}{32.6} &- &\textcolor{mdgreen}{85.0} &- &\textcolor{mdgreen}{59.6} &- &\textcolor{mdgreen}{3.4} &- \\
Mean &57.8 &1.7 &40.5 &15.1 &86.0 &0.9 &74.8 &10.3 &20.1 &8.0 \\\midrule
\textit{Ours(Roberta}) & & & & & & & & & & \\\midrule
Single &50.6 &5.5 &35.5 &10.1 &85.6 &0.5 &69.1 &4.6 &12.3 &0.2 \\
Upper. &\textcolor{red}{54.8} &- &\textcolor{red}{41.0 }&- &\textcolor{mdgreen}{86.3} &- &\textcolor{mdgreen}{80.1} &- &\textcolor{mdgreen}{22.1} &- \\
Lower. &\textcolor{red}{46.5} &- &\textcolor{red}{29.7} &- &\textcolor{mdgreen}{84.9} &- &\textcolor{mdgreen}{56.7} &- &\textcolor{mdgreen}{6.7} &- \\
Mean &50.6 &5.5 &35.4 &10.0 &85.6 &0.5 &68.4 &3.9 &14.4 &2.3 \\\midrule
Gold &56.1 &0.0 &25.4 &0.0 &85.1 &0.0 &64.5 &0.0 &12.1 &0.0 \\
\bottomrule
\end{tabularx}
\caption{Predicted test-set accuracy on semantic parsing tasks with LLaMA2 as the parser.
Green numbers refers to valid bounds that capture the gold accuracy.
Red numbers refer to the invalid bounds that cannot capture the gold accuracy.
}
\label{tab:app:llama_parser_sem_acc}
\end{table*}
