# Supplementary material for: Predicting generalization performance with correctness discriminators
Source: arXiv:2311.09422 source file (2025-05-21)
Supplement: Supplementary file 2 [file llama_parser_pos.tex]

\begin{table}[tb!]\centering
\footnotesize
\begin{tabularx}{\linewidth}{p{0.8cm}XXXXXX}\toprule
& \multicolumn{4}{c}{OOD} & \multicolumn{2}{c}{ID} \\
\cmidrule(lr){2-5}
\cmidrule(lr){6-7}
&\multicolumn{2}{c}{POS-Brown} &\multicolumn{2}{c}{POS-COGS} &\multicolumn{2}{c}{POS-WSJ} \\\cmidrule{2-7}
&Acc &AE &Acc &AE &Acc &AE \\
\midrule
{\textit{Ours(T5)}} \\\midrule
Single &58.6 &1.5 &85.9 &2.4 &60.5 &0.5 \\
Upper. &\textcolor{mdgreen}{79.0} &- &\textcolor{red}{87.0} &- &\textcolor{mdgreen}{79.9} &- \\
Lower. &\textcolor{mdgreen}{35.4} &- &\textcolor{red}{84.7} &- &\textcolor{mdgreen}{37.7} &- \\
Mean &57.2 &0.1 &85.8 &2.3 &58.8 &2.2 \\\midrule
{\textit{Ours(Vicuna})} \\\midrule
Single &49.6 &7.5 &81.9 &1.6 &53.5 &1.2 \\
Upper. &\textcolor{mdgreen}{82.0} &- &\textcolor{mdgreen}{88.7} &- &\textcolor{mdgreen}{84.6} &- \\
Lower. &\textcolor{mdgreen}{16.9} &- &\textcolor{mdgreen}{69.8} &- &\textcolor{mdgreen}{20.1} &- \\
Mean &49.5 &7.6 &79.3 &4.3 &52.3 &8.7 \\\midrule
{\textit{Ours(Roberta)}} \\\midrule
Single &58.2 &1.1 &88.0 &4.5 &61.2 &0.2 \\
Upper. &\textcolor{mdgreen}{82.1} &- &\textcolor{red}{89.5} &- &\textcolor{mdgreen}{84.1} &- \\
Lower. &\textcolor{mdgreen}{30.8} &- &\textcolor{red}{86.8} &- &\textcolor{mdgreen}{34.9} &- \\
Mean &56.4 &0.7 &88.2 &4.7 &59.5 &1.5 \\\midrule
Gold &57.1 &0.0 &83.5 &0.0 &61.0 &0.0 \\
\bottomrule
\end{tabularx}
\caption{Predicted accuracy on POS tagging tasks with LLaMA2 as the pos tagger.}
\label{tab:app:llama_parser_pos_acc}
\end{table}
