# Supplementary material for: Predicting generalization performance with correctness discriminators
Source: arXiv:2311.09422 source file (2025-05-21)
Supplement: Supplementary file 3 [file llama_parser_syn.tex]

\begin{table}[tb!]\centering
\footnotesize
\begin{tabularx}{\linewidth}{XXXXX}\toprule
&\multicolumn{2}{c}{OOD} &\multicolumn{2}{c}{ID} \\
\cmidrule(lr){2-3}
\cmidrule(lr){4-5}
&\multicolumn{2}{c}{Syn-Brown} &\multicolumn{2}{c}{Syn-WSJ} \\\cmidrule{2-5}
&Acc &AE &Acc &AE \\\midrule
{\textit{Ours(T5)}} \\\midrule
Single &45.9 &15.0 &54.0 &22.6 \\
Upper. &\textcolor{mdgreen}{68.2} &- &\textcolor{red}{74.7} &- \\
Lower. &\textcolor{mdgreen}{25.8} &- &\textcolor{red}{32.7} &- \\
Mean &47.0 &16.1 &53.7 &22.3 \\\midrule
{\textit{Ours(Vicuna)}} \\\midrule
Single &72.9 &42.0 &69.8 &38.4 \\
Upper. &\textcolor{red}{96.4} &- &\textcolor{red}{91.6} &- \\
Lower. &\textcolor{red}{36.8} &- &\textcolor{red}{40.1} &- \\
Mean &66.6 &35.7 &65.8 &34.4 \\\midrule
{\textit{Ours(Roberta})} \\\midrule
Single &42.0 &11.1 &47.7 &16.3 \\
Upper. &\textcolor{mdgreen}{75.2} & -&\textcolor{mdgreen}{79.2} &- \\
Lower. &\textcolor{mdgreen}{4.4} & -&\textcolor{mdgreen}{6.6} & -\\
Mean &39.8 &8.9 &42.9 &11.5 \\\midrule
Gold &30.9 &0.0 &31.4 &0.0 \\
\bottomrule
\end{tabularx}
\caption{Predicted accuracy on parsing tasks with LLaMA2 as the parser.}
\label{tab:app:llama_parser_syn_acc}
\end{table}
