# Supplementary material for: Predicting generalization performance with correctness discriminators
Source: arXiv:2311.09422 source file (2025-05-21)
Supplement: Supplementary file 4 [file roberta_pos.tex]

\begin{table}[tb!]\centering
\footnotesize
\begin{tabularx}{\linewidth}{p{0.8cm}XXXXXX}\toprule
& \multicolumn{4}{c}{OOD} & \multicolumn{2}{c}{ID} \\
\cmidrule(lr){2-5}
\cmidrule(lr){6-7}
&\multicolumn{2}{c}{POS-Brown} &\multicolumn{2}{c}{POS-COGS} &\multicolumn{2}{c}{POS-WSJ} \\\cmidrule{2-7}
&Acc &AE &Acc &AE &Acc &AE \\
\midrule
\multicolumn{7}{l}{\textit{Ours (Roberta)}} \\
\midrule
Single &50.5 &10.5 &86.9 &1.2 &54.2 &11.1 \\
Upper. &88.0 &- &87.6 &- &89.9 &- \\
Lower. &31.8 &- &86.1 &- &36.7 &- \\
Mean &59.9 &1.1 &86.8 &1.1 &63.3 &2.0 \\
\midrule
Gold &61.0 &0.0 &85.7 &0.0 &65.3 &0.0 \\
\bottomrule
\end{tabularx}
\caption{Predicted accuracy on POS tagging tasks.}
\label{tab:app:pos_acc}
\end{table}
