# Supplementary material for: Predicting generalization performance with correctness discriminators
Source: arXiv:2311.09422 source file (2025-05-21)
Supplement: Supplementary file 5 [file roberta_recall.tex]

\begin{table}[!htp]\centering
\scriptsize
\begin{tabularx}{\linewidth}{p{0.45cm}p{1.3cm}XXXXXX}\toprule
& &\multicolumn{2}{c}{Single} &\multicolumn{2}{c}{Upperbound} &\multicolumn{2}{c}{Lowerbound} \\
\cmidrule(lr){3-4}
\cmidrule(lr){5-6}
\cmidrule(lr){7-8}
& &CR &IR &CR &IR &CR &IR \\
\midrule
\multirow{7}{*}{OOD} &MCD1 &97 &90 &98.5 &80.8 &92.5 &97.3 \\
&MCD2 &78.3 &85 &84.7 &79.4 &70.6 &90.6 \\
&COGS &98.9 &87.7 &99.8 &86.6 &97.8 &90.8 \\
&TOP &85.4 &65.8 &91.3 &42.1 &77.7 &78.9 \\
&POS-Brown & 62.1 &67.4 &95.2 &23.3 &44.4 &88.0 \\
&POS-COGS &99.9 &90.9 &100.0 &86.7 &99.5 &94.9 \\
&Syn-Brown & 17.5 &74.3 &70.6 &38.4 &4.2 &96.3 \\
\midrule
\multirow{3}{*}{IID} &AMR 2.0 &38.9 &96.1 &59.1 &80.2 &37.3 &97.4 \\
&POS-WSJ &64.5 &65.2 &96.0 &21.7 &49.6 &87.6 \\
&Syn-WSJ & 27.1 &66 &74.3 &34.6 &6.5 &94.7 \\
\bottomrule
\end{tabularx}
\caption{Correct recall and incorrect recall scores of Roberta-based discriminators.}
\label{tab: app:roberta_recall}
\end{table}
