# Supplementary material for: Predicting generalization performance with correctness discriminators
Source: arXiv:2311.09422 source file (2025-05-21)
Supplement: Supplementary file 6 [file roberta_sem.tex]

\begin{table*}[tb!]\centering
\footnotesize
\begin{tabularx}{\linewidth}{XXXXXXXXXXX}
\toprule
& \multicolumn{8}{c}{OOD} & \multicolumn{2}{c}{ID} \\
\cmidrule(lr){2-9}
\cmidrule(lr){10-11}
&\multicolumn{2}{c}{MCD1} &\multicolumn{2}{c}{MCD2} &\multicolumn{2}{c}{COGS} &\multicolumn{2}{c}{TOP} &\multicolumn{2}{c}{AMR 2.0} \\\cmidrule{2-11}
&Acc &AE $\downarrow$ &Acc &AE $\downarrow$&Acc &AE $\downarrow$&Acc &AE $\downarrow$ &Acc &AE $\downarrow$\\\midrule
\multicolumn{11}{l}{\textit{Ours (Roberta)}} \\
\midrule
Single &60.2 &2.4 &29.5 &6.6 &91.4 &0.0 &71.6 &1.4 & 8.9& 5.4\\
Upper. &65.0 &- &35.3 &- &92.3 &- &82.3 &- & 25.5& -\\
Lower. &54.6 &- &23.4 &- &90.2 &- &62.4 &- & 7.6& -\\
Mean &59.8 &2.0 &29.3 &6.4 &91.3 &0.2 &72.3 &0.7 & 16.6& 2.3\\
\midrule

Gold &57.8 &0.0 &22.9 &0.0 &91.4 &0.0 &73.0 &0.0 &14.3 &0.0 \\
\bottomrule
\end{tabularx}
\caption{Predicted test-set accuracy with Roberta-based discriminators on semantic parsing tasks. 
}
\label{tab:app:sem_acc}
\end{table*}
