# Supplementary material for: Predicting generalization performance with correctness discriminators
Source: arXiv:2311.09422 source file (2025-05-21)
Supplement: Supplementary file 9 [file t5_recall.tex]

\begin{table}[!htp]\centering
\scriptsize
\begin{tabularx}{\linewidth}{p{0.45cm}p{1.3cm}XXXXXX}\toprule
& &\multicolumn{2}{c}{Single} &\multicolumn{2}{c}{Upperbound} &\multicolumn{2}{c}{Lowerbound} \\
\cmidrule(lr){3-4}
\cmidrule(lr){5-6}
\cmidrule(lr){7-8}
& &CR &IR &CR &IR &CR &IR \\
\midrule
\multirow{7}{*}{OOD} &MCD1 &97.0 &83.1 &99.2 &69.8 &92.9 &94.5 \\
&MCD2 &80.6 &83.7 &83.4 &77.9 &71.7 &92.2 \\
&COGS &98.5 &96.6 &99.8 &89.4 &98.5 &96.9 \\
&TOP &87.4 &57.9 &92.2 &44.7 &82.5 &78.9  \\
&POS-Brown &81.3 &54.7 &94.0 &26.0 &52.2 &84.7 \\
&POS-COGS &98.8 &86.3 &99.9 &84.4 &98.7 &89.2  \\
&Syn-Brown &33.8 &90.0 &69.3 &73.9 &29.7 &96.0 \\
\midrule
\multirow{3}{*}{ID} &AMR 2.0 &37.0 &98.3 &70.9 &84.1 &29.1 &99.1 \\
&POS-WSJ &80.2 &53.6 &93.0 &26.5 &52.4 &84.8  \\
&Syn-WSJ &44.5 &89.2 &66.2 &73.1 &20.5 &97.0  \\
\bottomrule
\end{tabularx}
\caption{Correct recall and incorrect recall scores of T5-based discriminators.}
\label{tab: app:recall}
\end{table}
