# Supplementary material for: Predicting generalization performance with correctness discriminators
Source: arXiv:2311.09422 source file (2025-05-21)
Supplement: Supplementary file 10 [file t5_sem.tex]

\begin{table*}[tb!]\centering
\footnotesize
\begin{tabularx}{\linewidth}{XXXXXXXXXXX}
\toprule
& \multicolumn{8}{c}{OOD} & \multicolumn{2}{c}{ID} \\
\cmidrule(lr){2-9}
\cmidrule(lr){10-11}
&\multicolumn{2}{c}{MCD1} &\multicolumn{2}{c}{MCD2} &\multicolumn{2}{c}{COGS} &\multicolumn{2}{c}{TOP} &\multicolumn{2}{c}{AMR 2.0} \\\cmidrule{2-11}
&Acc &AE $\downarrow$ &Acc &AE $\downarrow$&Acc &AE $\downarrow$&Acc &AE $\downarrow$ &Acc &AE $\downarrow$\\\midrule
\multicolumn{11}{l}{\textit{Ours (T5)}} \\
\midrule
Single & 63.1 &5.3 &31.0 &8.1 &90.3 &1.1 &75.2 &2.2 &6.0 &8.3 \\
Upper. &70.0 &- &{36.1} &- &92.1 &- &82.3 &- &18.3 &- \\
Lower. &56.0 &- &22.4 &- &90.2 &- &66.0 &- &3.4 &- \\
Mean &63.0 &{5.2} &29.3 &{6.4} &91.2 &{0.3} &74.2 &{1.2} &10.9 &{3.4} \\
\midrule

Gold &57.8 &0.0 &22.9 &0.0 &91.4 &0.0 &73.0 &0.0 &14.3 &0.0 \\
\bottomrule
\end{tabularx}
\caption{Predicted test-set accuracy with T5-based discriminators on semantic parsing tasks. 
}
\label{tab:app:sem_acc}
\end{table*}
