# Supplementary material for: Predicting generalization performance with correctness discriminators
Source: arXiv:2311.09422 source file (2025-05-21)
Supplement: Supplementary file 11 [file t5_syn.tex]

\begin{table}[tb!]\centering
\footnotesize
\begin{tabularx}{\linewidth}{XXXXX}\toprule
&\multicolumn{2}{c}{OOD} &\multicolumn{2}{c}{ID} \\
\cmidrule(lr){2-3}
\cmidrule(lr){4-5}
&\multicolumn{2}{c}{Syn-Brown} &\multicolumn{2}{c}{Syn-WSJ} \\\cmidrule{2-5}
&Acc &AE &Acc &AE \\\midrule
\multicolumn{5}{l}{\textit{Ours (T5)}} \\\midrule
Single &38.1 &4.3 &45.0 &7.4 \\
Upper. &57.5 &- &64.2 &- \\
Lower. &17.9 &- &24.6 &- \\
Mean &37.7 &3.9 &44.4 &6.8 \\
\midrule
Gold &33.8 &0.0 &37.6 &0.0 \\
\bottomrule
\end{tabularx}
\caption{Predicted accuracy on parsing tasks.}
\label{tab:app:syn_acc}
\end{table}
